# Supplementary material for: Skill over Scale: The Case for Medium, Domain-Specific Models for SE
Source: arXiv:2306.03268 source file (2025-02-21)
Supplement: Supplementary file 1 [file Appendix.tex]

\newpage
\section{Appendix -- Ignore this is supplemntary material}

\subsection{Zero shot prompts}

\begin{lstlisting}
The Text below is a StackOverflow answer or comment on an answer. Your task is to determine if this text includes any mentions of obsolete code. This includes comments pointing out obsolete code in the answer, or answers edited to point out they contain or previously contained outdated solutions. Generate the label 1 if the text shown matches this definition and 0 if it does not.

Text: {PLACEHOLDER}
Label:

\end{lstlisting}

\subsection{10 shot prompt + CoT}

\begin{lstlisting}
The Text below is a StackOverflow answer or comment on an answer. Your task is to determine if this text includes any mentions of obsolete code. This includes comments pointing out obsolete code in the answer, or answers edited to point out they contain or previously contained outdated solutions. First emit a rationale following the examples below. Then, generate the label 1 if the text shown matches this definition and 0 if it does not.

Text: @Alp I believe DOM2 Mutation Events have been [replaced by DOM4 Mutation Observers](https://code.google.com/p/chromium/issues/detail?id=142648) in recent builds. [Try this article](http://updates.html5rocks.com/2012/02/Detect-DOM-changes-with-Mutation-Observers).
Rationale: This text doesn't mention any code with obsoletion.
Label: 0

Text: The first and second screenshots you posted show an error from aapt2 that you got during mergeDebugResources task.	
Rationale: This text doesn't mention any code with obsoletion.
Label: 0

Text: The question is not about ASP.NET MVC Core (and it did not even exist at the time the question was asked)
Rationale: This text doesn't mention any code with obsoletion.
Label: 0

Text: There are various ways to get a MediaStream which is originating from gUM, but you won't be able to catch all possible audio output...\nBut, for your mp3 file, if you read it through an MediaElement (<code> <audio> </code> or <code> <video> </code> ), and if this file is served without breaking CORS, then you can use <code> MediaElement.captureStream </code> .\nIf you read it from WebAudioAPI, or if you target browsers that don't support <code> captureStream </code> , then you can use AudioContext.createMediaStreamDestination.\nFor SpeechSynthesis, unfortunately you will need gUM... and a Virtual Audio Device: first you would have to set your default output to the VAB_out, then route your VAB_out to VAB_in and finally grab VAB_in from gUM... \nNot an easy nor universally doable task, moreover when IIRC SpeechSynthesis doesn't have any setSinkId method.\n	
Rationale: This text doesn't mention any code with obsoletion.
Label: 0

Text: can you, please, extent you answer with adding the types explicitly to the vars? thank you!
Rationale: This text doesn't mention any code with obsoletion.
Label: 0

Text: That explains it. I had this vague memory of things being different in XCode 2.5 and 3.0	
Rationale: Also this mentions some versions, this text doesn't mention any code with obsoletion.
Label: 0

Text: yes, there is a way to take the first value automatically, however, it's not obvious. gnuplot has no function, e.g. like a = value(row,column), but there is a workaround. I will adapt the code.	
Rationale: This text doesn't mention any code with obsoletion.
Label: 0

Text: @JuanCarlosVerdeCortez please post it as a new question, including all the details in the question body (not title or comments), it will increase your chances of someone helping you to solve the problem. ...or simply try to search for an answer - looks like MethodInvokingTimerTaskFactoryBean was deprecated as of Spring 3.	
Rationale: This mentions that MethodInvokingTimerTaskFactoryBean was deprecated as of Spring 3.
Label: 1

Text: I think now the API changes to <code> MongoDB\BSON\ObjectID </code> , also you can use <code> [] </code> to denote an array in PHP 5.4+, so it should be:\n<code> 
collection->findOne(['_id' => new MongoDB\BSON\ObjectID( idToken )]);\n </code> \nbased on Phil's answer.\n
Rationale: This mentions changes  API changes to <code> in PHP 5.4+.
Label: 1

Text: For those reading this super constructor is now deprecated. super(AppUnderTest.class) should be sufficient
Rationale: This mentions the super constructor being deprecated.
Label: 1

Text: {PLACEHOLDER}
Rationale:


\end{lstlisting}
